# Supplementary material for: A Mixture-Based Framework for Guiding Diffusion Models
Source: arXiv:2502.03332 source file (2025-02-05)
Supplement: Supplementary file 1 [file apdx.tex]

\section{You \emph{can} have an appendix here.}
