# Supplementary material for: A Mixture-Based Framework for Guiding Diffusion Models
Source: arXiv:2502.03332 source file (2025-02-05)
Supplement: Supplementary file 2 [file gauss_case.tex]

\section{Gaussian case}

% --- local vars ---
\def\cov{\mathbf{\Sigma}}
\def\mean{\boldsymbol{m}}
\def\likelihood{\bfA}

\def\potBias{\boldsymbol{a}}
\def\potLikelihood{\hat{\likelihood}}

\def\LH{\mathbf{H}}
\def\Lbias{\boldsymbol{h}}
\def\Lcov{\mathbf{L}}

\def\LHbefore{\underline{\mathbf{H}}}
\def\Lbiasbefore{\underline{\boldsymbol{h}}}
\def\Lcovbefore{\underline{\mathbf{L}}}

\def\pizero{\mathbf{M}}
\def\pik{\mathbf{N}}
\def\picov{\mathbf{\Lambda}}
\def\pibias{\boldsymbol{e}}

\def\covtau{\mathbf{\Sigma}_{\bx}}
\def\meantau{\boldsymbol{\mu}_{\bx}}

\def\matzero{\mathbf{C}}
\def\biaszero{\boldsymbol{c}}
\def\covzero{\mathbf{\Sigma}_{c}}

\def\matk{\mathbf{D}}
\def\biask{\boldsymbol{d}}
\def\covk{\mathbf{\Sigma}_{d}}

\def\covthree{\mathbf{\Psi}}
\def\centeredxzero{\bar{\bx}_0'}
\def\centeredxk{\bar{\bx}_k'}

% no need for theta as superscript of the potential
\renewcommand{\hpotn}[2]{\ifthenelse{\equal{#2}{}}{\hat{g} _{#1}}{\hat{g} _{#1}(#2)}}
% ---

Recall that in this setting, the
\begin{itemize}
    \item prior is a Gaussian $\prior = \gauss(\mean, \cov)$, where $(\mean, \cov) \in \rset^\dimx \times \mathcal{S}^{++} _\dimx$
    \item potential is the likelihood of a linear inverse problem $\potn{}{}: \bx \mapsto \normpdf(\obs; \bfA \bx, \stdobs^2 \Id_\dimobs)$
\end{itemize}
% In the setting where the prior is a Gaussian $\prior = \gauss(\mean, \cov)$
% and the potential is the likelihood of a linear inverse problem $\potn{}{}: \bx \mapsto \normpdf(\obs; \bfA \bx, \stdobs^2 \Id_\dimobs)$,
In such a setting, all random variables involved in \Cref{algo:midpoint-gibbs} are Gaussians and hence the algorithm reduces to a sequence of means and covariances.
Depending on the number of gibbs repetitions $\gibbsReps$, \Cref{algo:midpoint-gibbs} simulates a final distribution $\pibw{0}{}{}[\gibbsReps]$.

In this section, we derive the recursion verified by the means and covariances of $\{ \pibw{k}{}{}[\gibbsReps] \}_{0 \leq k \leq n}$.
We proceed by:
% (i) writing the denoising densitites $\{ \bw{\initpoint|k}{}{} \}_{0 \leq k \leq n}$ and the approximate potentials $\{ \hpotn{k}{} \}_{0 \leq k \leq n}$ in the case of $\prior$ gaussian, (ii) deriving the transition kernels in \Cref{apdx:transition-kernels} in that case, (iii) combining the results to form the the recursion.
\begin{enumerate}
    \item writing the denoising densitites $\{ \bw{\initpoint|k}{}{} \}_{0 \leq k \leq n}$ and the approximate potentials $\{ \hpotn{k}{} \}_{0 \leq k \leq n}$
    \item deriving the transition kernels in \Cref{apdx:transition-kernels} in that case
    \item combining the results to form the the recursion
\end{enumerate}

\paragraph{Denoising densities and potentials.} Since we are dealing with a Gaussian prior, the denoiser $\predx{k}$ can be computed in closed form for any $k \in \intset{1}{n}$. Using \citet[Eqn.~2.116]{bishop2006pattern}, we have that
    \begin{align*}
        \bw{0|k}{\bx _k}{\bx _0}
            & \propto \prior(\bx _0) \fwtrans{k|0}{\bx _0}{\bx _k} \\
            & = \normpdf \big(\bx _0;
                \cov_{0|k} \big( (\sqrt{\acp{k}} / \var_k) \bx _k + \cov^{-1} \mean \big), \cov_{0|k} \big),
    \end{align*}
where $\cov_{0|k} \eqdef ((\acp{k} / \var_k) \Id + \cov^{-1})^{-1}$.
A byproduct is an expression of the denoiser
\begin{equation*}
    \predx{k}(\bx _k) = \cov_{0|k}\big( (\sqrt{\acp{k}} / \var_k) \bx _k + \cov^{-1} \mean \big)
    \eqsp.
\end{equation*}

The approximate potentials $\hpotn{k}{} = \potn{k}{} \circ \predx{k}$ also have an explicit expression that reads
\begin{equation*}
    \hpotn{k}{\bx _k}
        = \normpdf(\obs; \hat\bfA_k \bx _k + \potBias_k, \stdobs^2 \Id_\dimobs),
    \quad
    \mathrm{where}
    \quad
    \potLikelihood_k = (\sqrt{\acp{k}} / \var_k)  \likelihood \cov_{0|k}, \quad \potBias_k = \likelihood \cov_{0|k} \cov^{-1} \mean
    \eqsp.
\end{equation*}

\paragraph{Transition kernels.}
The expression of the initial kernel \eqref{eq:gibbs-init-kernel} writes
\begin{equation*}
    % \label{eq:init-kernel-gauss}
    \initKernel(\bx_\initpoint; \rmd \bx_\initpoint', \rmd \bx_k')
        = \delta_{\bx_\initpoint}(\rmd \bx_\initpoint')
            \ \normpdf(\rmd \bx_k'; \sqrt{\acp{k}} \bx_0, \var_{k} \Id_\dimx)
    \eqsp.
\end{equation*}
This can be translated into the following linear system of random variables
\begin{align*}
    \bX_0' 
        & = \bX_0,
        \\
    \bX_k' 
        & = \sqrt{\acp{k}} \bX_0 + \sqrt{\var_k} \bZ, 
        \qquad \bZ \sim \normpdf(\zero, \Id_\dimx).
\end{align*}
Notice here that $\bX_0'$ and $\bX_k'$ of the next state are interlinked
$\pCov[\bX_0', \bX_k'] = \sqrt{\acp{k}} \pV[\bX_0]$, an that
\begin{equation}
    \label{eq:gibbs-init-kernel-gauss-update}
    \pE\begin{bmatrix}\bX_0'\\\bX_k'\end{bmatrix} = \begin{bmatrix}\pE[\bX_0]\\\sqrt{\acp{k}}\pE[\bX_0]\end{bmatrix},
    \quad
    \pCov\begin{bmatrix}\bX_0'\\\bX_k'\end{bmatrix} = \begin{bmatrix}\pV[\bX_0] & \sqrt{\acp{k}}\pV[\bX_0]\\\cdot & \var_{k} \Id_\dimx + \acp{k} \pV[\bX_0]\end{bmatrix}
    \eqsp.
\end{equation}

It is easy to see that \Cref{eq:gibbs-kernel-one-rep} can also be expressed as a linear system of random variables
% \begin{equation}
%     \label{eq:gibbs-kernel-one-rep-gauss}
%     \gibbsRepKernel(\bx_{\initpoint}, \bx_k; \rmd \bx_{\initpoint}', \rmd \bx_k')
%         = \normpdf(\rmd \bx_{\initpoint}';
%             \QMzero_k \bx_0 + \QNzero_k \bx_k + \Qbiaszero_k, \Qcovzero_k) \
%             \normpdf(\rmd \bx_k'; \QMk_k \bx_0 + \QNk_k \bx_k + \Qbiask_k, \Qcovk_k)
%     \eqsp.
% \end{equation}
% \begin{align*}
%     \bX_0' 
%         & = \QMzero_k \bX_0 + \QNzero_k \bX_k + \Qbiaszero_k + \Qcovzero_k^{1/2} \bZ_0,
%         \qquad \bZ_0 \sim \normpdf(\zero, \Id),
%         \\
%     \bX_k' 
%         & = \QMk_k \bX_0 + \QNk_k \bX_k + \Qbiask_k + \Qcovk_k^{1/2} \bZ_k, 
%         \qquad \bZ_k \sim \normpdf(\zero, \Id).
% \end{align*}
\begin{equation*}
    \begin{bmatrix}\bX_0'\\\bX_k'\end{bmatrix}
    =
    \boldsymbol{b}_k
    + 
    \mathbf{B}_k \begin{bmatrix}\bX_0\\\bX_k\end{bmatrix}
    +
    \mathbf{\Gamma}^{1/2}_k \bZ_{0,k}
    , \quad
    \bZ_{0,k} \sim \normpdf(\zero_{2\dimx}, \Id_{2\dimx})
    \eqsp.
\end{equation*}
For clarity, we defer the expressions of the introduced matrices $\mathbf{B}_k, \mathbf{\Gamma}_k$, and the bias $\boldsymbol{b}_k$ to \Cref{apdx:details-expressions-gauss}.
Based on the values of expected value of the vector $[\bX_0, \bX_k]$ and its covariance, we can deduce the expected value and the covariances of the next state $\bX_0', \bX_k'$ as follow
\begin{equation}
    \label{eq:gibbs-kernel-one-rep-gauss}
    \pE\begin{bmatrix}\bX_0'\\\bX_k'\end{bmatrix}
        =
        \boldsymbol{b}_k
        + 
        \mathbf{B}_k \ \pE\begin{bmatrix}\bX_0\\\bX_k\end{bmatrix},
    \quad
    \pCov\begin{bmatrix}\bX_0'\\\bX_k'\end{bmatrix}
        = 
        \mathbf{B}_k \pCov\begin{bmatrix}\bX_0\\\bX_k\end{bmatrix} \mathbf{B}_k^\top + \mathbf{\Gamma}_k
    \eqsp.
\end{equation}
% For clarity, we defer the expressions of the introduced matrices $\QMzero_k, \QNzero_k, \Qcovzero_k$, and $\QMk_k, \QNk_k, \Qcovk_k$, and the biases $\Qbiaszero_k, \Qbiask_k$ to \Cref{apdx:details-expressions-gauss}.
% The expression of the initial kernel \eqref{eq:gibbs-init-kernel} writes
% \begin{equation}
%     \label{eq:init-kernel-gauss}
%     \initKernel(\bx_\initpoint; \rmd \bx_\initpoint', \rmd \bx_k')
%         = \delta_{\bx_\initpoint}(\rmd \bx_\initpoint')
%             \ \normpdf(\rmd \bx_k'; \sqrt{\acp{k}} \bx_0, \var_{k} \Id_\dimx)
%     \eqsp.
% \end{equation}
Finally, the last kernel \eqref{eq:algo-last-kernel} is a Gaussian with a linear mean on $\bx_2$
\begin{equation*}
    \lastKernel(\bx_2; \rmd \bx_0') = \normpdf(\rmd \bx_0'; \LH \bx_2 + \Lbias, \Lcov)
    \eqsp.
\end{equation*}
Also here for clarity, we defer the expressions of the introduced matrices $\LH, \Lcov$ and the bias  $\Lbias$ to \Cref{apdx:details-expressions-gauss}.
Therefore, we deduce the updates
\begin{equation}
    \label{eq:last-kernel-gauss}
    \pE[\bX_0'] = \LH \pE[\bX_2] + \Lbias,
    \quad
    \pV[\bX_0'] = \LH \pV[\bX_2] \LH^\top + \Lcov
    \eqsp.
\end{equation}

\paragraph{Recursion.}
By combining \eqref{eq:gibbs-init-kernel-gauss-update}, \eqref{eq:gibbs-kernel-one-rep-gauss}, and \eqref{eq:last-kernel-gauss}, \Cref{algo:midpoint-gibbs} reduces to the following recursion
% \badr{here the init $\delta_m(\rmd \bx_0^n)$ is valid if we were in the perfect case where the diffusion converges to a Gaussian}
% \begin{equation*}
%     \begin{aligned}
%         \pE[\bX_0^{(0)}] = \bx_0, \pV[\bX_0^{(0)}] = \zero,
%             \quad & \quad
%         \pE[\bX_k^{(0)}] = \sqrt{\acp{k}} \bx_0, \pV[\bX_k^{(0)}] = \var_{k} \Id_\dimx, \\
%         \pE[\bX_0^{(r+1)}] = \QMzero_k \pE[\bX_0^{(r)}] + \QNzero_k \pE[\bX_k^{(r)}],
%             \quad & \quad
%         \pV[\bX_0^{(r+1)}] = \Qcovzero_k + \QMzero_k  \pV[\bX_0^{(r)}] \QMzero_k^\top + \QNzero_k \pV[\bX_k^{(r)}] \QNzero_k^\top,
%         \\
%         \pE[\bX_k^{(r+1)}] = \QMk_k \pE[\bX_0^{(r)}] + \QNk_k \pE[\bX_k^{(r)}],
%             \quad & \quad
%         \pV[\bX_k^{(r+1)}] = \Qcovk_k + \QMk_k \pV[\bX_0^{(r)}] \QMk_k^\top + \QNk_k \pV[\bX_k^{(r)}] \QNk_k^\top,
%     \end{aligned}
% \end{equation*}
\begin{algorithm}[h]
    \caption{\Cref{algo:midpoint-gibbs} in the Gaussian case}
    \begin{algorithmic}[1]
        \STATE $\pE[\bX_{\initpoint}^n] \gets \mean,
            \quad
            \pV[\bX_{\initpoint}^n] \gets \zero$
        \FOR{$k=n-1$ to $2$}
            % \STATE {\bfseries Pick:} $\midpoint \sim \uniform(\intset{1}{k-1})$
            % \STATE {\bfseries Init:} $\bX^{(0)}_k \sim \fwtrans{k|0}{\bX_{\initpoint}}{\cdot}, \, \bX^{(0)}_{\initpoint} \gets \bX_{\initpoint}$

            % \STATE $\pE[\bX_0^{(0)}] \gets \pE[\bX_0^{k+1}],
            % \quad
            % \pV[\bX_0^{(0)}] \gets  \pV[\bX_0^{k+1}]$
            % \STATE $\pE[\bX_k^{(0)}] \gets \sqrt{\acp{k}} \ \pE[\bX_0^{k+1}],
            % \quad
            % \pV[\bX_k^{(0)}] \gets \var_{k} \Id_\dimx + \acp{k} \pV[\bX_0^{k+1}]$
            % \STATE $\pCov[\bX_0^{(0)}, \bX_k^{(0)}] \gets \sqrt{\acp{k}} \pV[\bX_0^{k+1}]$
            
            \STATE $\pE\begin{bmatrix}\bX_0^{(0)}\\\bX_k^{(0)}\end{bmatrix} \gets \begin{bmatrix}\pE[\bX_0^{k+1}]\\\sqrt{\acp{k}}\pE[\bX_0^{k+1}]\end{bmatrix},$ \qquad
            $\pCov\begin{bmatrix}\bX_0^{(0)}\\\bX_k^{(0)}\end{bmatrix} \gets \begin{bmatrix}\pV[\bX_0^{k+1}] & \sqrt{\acp{k}}\pV[\bX_0^{k+1}]\\\cdot & \var_{k} \Id_\dimx + \acp{k} \pV[\bX_0^{k+1}]\end{bmatrix}$

            \FOR{$r = 0$ {\bfseries to} $R-1$}
                % \STATE $\pE[\bX_0^{(r+1)}] \gets \QMzero_k \pE[\bX_0^{(r)}] + \QNzero_k \pE[\bX_k^{(r)}] + \Qbiaszero_k,
                % \quad
                % \pV[\bX_0^{(r+1)}] \gets \Qcovzero_k + \QMzero_k  \pV[\bX_0^{(r)}] \QMzero_k^\top + \QNzero_k \pV[\bX_k^{(r)}] \QNzero_k^\top$
                % \STATE $\pE[\bX_k^{(r+1)}] \gets \QMk_k \pE[\bX_0^{(r)}] + \QNk_k \pE[\bX_k^{(r)}] + \Qbiask_k,
                % \quad
                % \pV[\bX_k^{(r+1)}] \gets \Qcovk_k + \QMk_k \pV[\bX_0^{(r)}] \QMk_k^\top + \QNk_k \pV[\bX_k^{(r)}] \QNk_k^\top$
                % \STATE \emph{Apply \Cref{eq:gibbs-kernel-one-rep-gauss} starting from $\pE[\bX_0^{(r)}], \pE[\bX_k^{(r)}], \pV[\bX_0^{(r)}], \pV[\bX_k^{(r)}]$ and $\pCov[\bX_0^{(r)}, \bX_k^{(r)}]$}
                % \STATE \emph{to compute $\pE[\bX_0^{(r+1)}], \pE[\bX_k^{(r+1)}], \pV[\bX_0^{(r+1)}], \pV[\bX_k^{(r+1)}]$ and $\pCov[\bX_0^{(r+1)}, \bX_k^{(r+1)}]$}
                
                \STATE $\pE\begin{bmatrix}\bX_0^{(r+1)}\\\bX_k^{(r+1)}\end{bmatrix}
                \gets
                \boldsymbol{b}_k
                + 
                \mathbf{B}_k \ \pE\begin{bmatrix}\bX_0^{(r)}\\\bX_k^{(r)}\end{bmatrix}$,
                \qquad
                $\pCov\begin{bmatrix}\bX_0^{(r+1)}\\\bX_k^{(r+1)}\end{bmatrix}
                \gets 
                \mathbf{B}_k \pCov\begin{bmatrix}\bX_0^{(r)}\\\bX_k^{(r)}\end{bmatrix} \mathbf{B}_k^\top + \mathbf{\Gamma}_k$
                
            \ENDFOR
            \STATE $\pE[\bX_{\initpoint}^k] \gets \pE[\bX^{(R)}_{\initpoint}],
            \quad
            \pV[\bX_{\initpoint}^k] \gets \pV[\bX^{(R)}_{\initpoint}]$
            \STATE $\pE[\bX_k] \gets \pE[\bX^{(R)}_k],
            \quad
            \pV[\bX_k] \gets \pV[\bX^{(R)}_k]$
        \ENDFOR

        \STATE $\pE[\bX_0] \gets \LH \ \pE[\bX_2] + \Lbias
        \quad
        \pV[\bX_0] \gets \Lcov + \LH \ \pV[\bX_2] \ \LH^\top$
    \end{algorithmic}
\end{algorithm}

\paragraph{Expressions of the introduced matrices and biases.}
\label{apdx:details-expressions-gauss}
To derive the expression, we utilize \citet[Eqn.~2.116]{bishop2006pattern} and the convolution of two Gaussians.
Let us start we the kernel $\gibbsRepKernel$ \eqref{eq:gibbs-kernel-one-rep-gauss}.
We have
\begin{equation*}
    \begin{aligned}
        \mgibbs{\midpoint |\initpoint, k}{\bx_\initpoint, \bx_k}{\bx_{\midpoint}}
            & \propto \hpotn{\midpoint}{\bx _\midpoint} \fwtrans{\midpoint |\initpoint, k}{\bx_\initpoint, \bx_k}{\bx_{\midpoint}}\\
            & \propto \normpdf(\obs; \hat\bfA_\midpoint \bx _\midpoint + \potBias_\midpoint, \stdobs^2 \Id_\dimobs)
                \ \normpdf(\bx_{\midpoint}; \meanBridge_{\midpoint|0, k}(\bx _0, \bx _k), \var_{\midpoint|0, k} \Id_\dimx) \\
            & = \normpdf(\bx_\tau;
                \pizero_{\midpoint| 0, k} \bx_0 + \pik_{\midpoint| 0, k} \bx_k + \pibias_{\midpoint| 0, k},
                % var
                \picov_{\midpoint| 0, k})
    \end{aligned}
\end{equation*}
where
\begin{align*}
    \picov_{\midpoint|0, k}
        & = \big[ (1 /\var_{\midpoint | 0, k}) \Id_\dimx  + (1 / \stdobs^2)\hat\bfA_\midpoint^\top \hat\bfA_\midpoint \big]^{-1},\\
    \pizero_{\midpoint| 0, k}
        & = \frac{\sqrt{\acp{\midpoint}{} / \acp{0}}(1 - \acp{k} / \acp{\midpoint})}{\var_{\midpoint|0, k} (1 - \acp{k} / \acp{0})} \picov_{\midpoint| 0, k}
    ,\qquad
    \pik_{\midpoint| 0, k}
        = \frac{\sqrt{\acp{k} / \acp{\midpoint}} (1 - \acp{\midpoint} / \acp{0})}{\var_{\midpoint|0, k} (1 - \acp{k} / \acp{0})}  \picov_{\midpoint| 0, k}, \\
    \pibias_{\midpoint| 0, k}
        & = (1/\stdobs^2) \picov_{\midpoint| 0, k} \hat\bfA_\midpoint^\top (\obs - \potBias_\midpoint).\\
\end{align*}
After establishing the the distribution $\mgibbs{\midpoint |\initpoint, k}{}{}$, we can now compute the action of the kernel $\gibbsRepKernel$ on $\bX_0, \bX_k$.
Without lost of generality, we can write the integral involved in $\gibbsRepKernel$ as
\begin{align*}
    \int
        \mgibbs{\midpoint |\initpoint, k}{\bx_\initpoint, \bx_k}{\bx_{\midpoint}}
        \mgibbs{\initpoint |\midpoint}{\bx_{\midpoint}}{\bx_\initpoint'}
        \mgibbs{k |\midpoint}{\bx_{\midpoint}}{\bx_k'} \rmd \bx_\tau
        & = \int
            \normpdf(\bx_\tau; \meantau, \covtau)
            \normpdf(\bx_0'; \matzero \bx_\tau + \biaszero, \covzero)
            \normpdf(\bx_k'; \matk \bx_\tau + \biask, \covk)
            \rmd \bx_\tau
\end{align*}
where
\begin{align*}
    \meantau = \pizero_{\midpoint| 0, k} \bx_0 + \pik_{\midpoint| 0, k} \bx_k + \pibias_{\midpoint| 0, k}, \quad
    \covtau = \picov_{\midpoint|0, k},
    \\
    \matzero = (\sqrt{\acp{\tau}}/\var_{\tau}) \cov_{0|\tau}, \quad 
    \biaszero = \cov_{0|\tau} \cov^{-1} \mean, \quad
    \covzero = \cov_{0 | \tau},
    \\
    \matk = \sqrt{\acp{k}/\acp{\tau}} \Id, \quad 
    \biask = \zero, \quad
    \covk = \var_{k|\tau} \Id.
\end{align*}
From now on, we can focus only the quadratic product in the Gaussians exponent.
We have
\begin{multline*}
    \| \bx_\tau - \meantau \|^2_{\covtau^{-1}}
    +  \| \bx_0' - (\matzero \bx_\tau + \biaszero) \|^2_{\covzero^{-1}}
    + \| \bx_k' - (\matk \bx_\tau + \biask) \|^2_{\covk^{-1}}
    = 
    \\
    \| \bx_\tau \|^2_{\covtau^{-1} + \matzero^\top \covzero^{-1} \matzero + \matk^\top \covk^{-1} \matk}
    \\
    - 2 \langle \covtau^{-1} \meantau + \matzero^\top \covzero^{-1} (\bx_0'- \biaszero)+ \matk^\top \covk^{-1} (\bx_k'- \biask), \bx_\tau  \rangle
    \\
    + \| \meantau \|^2_{\covtau^{-1}} + \| \bx_0' - \biaszero \|^2_{\covzero^{-1}} + \| \bx_k' - \biask \|^2_{\covk^{-1}}
\end{multline*}
For the sake of conciseness, denote by
\begin{align*}
    \covthree^{-1} 
        & = \covtau^{-1} + \matzero^\top \covzero^{-1} \matzero + \matk^\top \covk^{-1} \matk,
        \\
    \centeredxzero & = \bx_0' - \biaszero, \qquad
    \centeredxk  = \bx_k' - \biask.
\end{align*}
The previous quadratic sum equal up to a constant independent of $\bx_\tau, \centeredxzero, \centeredxk$, to
\begin{align*}
    \| \bx_\tau - \covthree (\covtau^{-1} \meantau + \matzero^\top \covzero^{-1} \centeredxzero + \matk^\top \covk^{-1} \centeredxk) \|^2_{\covthree^{-1}}
    + \| \centeredxzero \|^2_{\covzero^{-1}} + \| \centeredxk \|^2_{\covk^{-1}}
    - \| \covtau^{-1} \meantau + \matzero^\top \covzero^{-1} \centeredxzero + \matk^\top \covk^{-1} \centeredxk \|^2_{\covthree}
    % \eqsp.
\end{align*}
The first term will define a Gaussian on $\bx_\tau$ and hence will integrate to one.
Hence, we get ride of the integration and will be left three terms.
The goal is to write them in form amenable to Gaussians.
Building up the previous expression, we have
\begin{multline*}
    \| \centeredxzero \|^2_{\covzero^{-1}} + \| \centeredxk \|^2_{\covk^{-1}}
    - \| \covtau^{-1} \meantau + \matzero^\top \covzero^{-1} \centeredxzero + \matk^\top \covk^{-1} \centeredxk \|^2_{\covthree}
    = \\
    \| \centeredxzero \|^2_{\covzero^{-1} - \covzero^{-1} \matzero \covthree \matzero^\top \covzero^{-1}} 
    + \| \centeredxk \|^2_{\covk^{-1} - \covk^{-1} \matk \covthree \matk^\top \covk^{-1}}
    \\
    - 2 \langle \matzero^\top \covzero^{-1} \centeredxzero, \matk^\top \covk^{-1} \centeredxk \rangle_{\covthree}
    - 2 \langle \covtau^{-1} \meantau, \matzero^\top \covzero^{-1} \centeredxzero \rangle_{\covthree}
    - 2 \langle \covtau^{-1} \meantau, \matk^\top \covk^{-1} \centeredxk \rangle_{\covthree}
\end{multline*}
where the equality is up to a constant independent of $\centeredxzero, \centeredxk$.

Now let us introduce the block matrices
\begin{equation*}
    \begin{aligned}
        \mathbf{\Gamma}^{-1} & = \begin{bmatrix}
            \covzero^{-1} - \covzero^{-1} \matzero \covthree \matzero^\top \covzero^{-1} &  -\covzero^{-1} \matzero \covthree \matk^\top \covk^{-1} \\
            \cdot & \covk^{-1} - \covk^{-1} \matk \covthree \matk^\top \covk^{-1}
        \end{bmatrix}
        \\
        \mathbf{J} & = \begin{bmatrix}
            \covzero^{-1} \matzero \covthree \covtau^{-1} & \zero \\
            \zero &  \covk^{-1} \matk \covthree \covtau^{-1} 
        \end{bmatrix}
    \end{aligned}
    \eqsp,
\end{equation*}
where the "$\cdot$" in the the expression of $\mathbf{\Gamma}^{-1}$ stands for the transpose of the off-diagonal element.
It follows that we can rewrite the previous equation in blocks as
\begin{align*}
    \begin{bmatrix}\centeredxzero \\ \centeredxk \end{bmatrix}^\top
    \mathbf{\Gamma}^{-1}
    \begin{bmatrix}\centeredxzero \\ \centeredxk \end{bmatrix}
    - 2 \langle
        \mathbf{J} \begin{bmatrix}\meantau \\ \meantau \end{bmatrix}
        ,
        \begin{bmatrix}\centeredxzero \\ \centeredxk \end{bmatrix}
    \rangle
    = 
    \| 
        \begin{bmatrix}\centeredxzero \\ \centeredxk \end{bmatrix} 
        -
        \mathbf{\Gamma} \mathbf{J} \begin{bmatrix}\meantau \\ \meantau \end{bmatrix}
    \|_{\mathbf{\Gamma}^{-1}}^2
    \eqsp,
\end{align*}
where the equality is up to a constant independent of $\centeredxzero, \centeredxk$.
Therefore, we can deduce that the random vector $[\bX_0', \bX_k']^\top$ is Gaussian as follows
\begin{equation*}
    \begin{aligned}
       \begin{bmatrix}\bX_0'\\\bX_k'\end{bmatrix}
       \sim
       \normpdf(
            \begin{bmatrix}\biaszero\\\biask\end{bmatrix}
            + \mathbf{\Gamma} \mathbf{J} \begin{bmatrix}\meantau \\ \meantau\end{bmatrix}
            ,
            \mathbf{\Gamma}
       )
    \end{aligned}
\end{equation*}
We can now intervene $\bX_0, \bX_k$ by subtituting with the value of $\meantau$
\begin{align*}
    \begin{bmatrix}\meantau \\ \meantau\end{bmatrix}
        = \begin{bmatrix}
            \pizero_{\midpoint| 0, k} & \pik_{\midpoint| 0, k}\\ 
            \pizero_{\midpoint| 0, k} & \pik_{\midpoint| 0, k} 
        \end{bmatrix} 
        \begin{bmatrix}\bX_0 \\ \bX_k\end{bmatrix}
        +
        \begin{bmatrix}\pibias_{\midpoint| 0, k} \\ \pibias_{\midpoint| 0, k}\end{bmatrix}
        = \mathbf{K} \begin{bmatrix}\bX_0 \\ \bX_k\end{bmatrix} + \begin{bmatrix}\pibias_{\midpoint| 0, k} \\ \pibias_{\midpoint| 0, k}\end{bmatrix}
\end{align*}
and therefore, we can write
\begin{equation*}
    \begin{aligned}
       \begin{bmatrix}\bX_0'\\\bX_k'\end{bmatrix}
       =
        \begin{bmatrix}\biaszero\\\biask\end{bmatrix}
        + 
        \mathbf{\Gamma} \mathbf{J} \begin{bmatrix}\pibias_{\midpoint| 0, k} \\ \pibias_{\midpoint| 0, k}\end{bmatrix}
        + 
        \mathbf{\Gamma} \mathbf{J} \mathbf{K} \begin{bmatrix}\bX_0\\\bX_k\end{bmatrix}
        +
        \mathbf{\Gamma}^{1/2} \bZ
    \end{aligned}
\end{equation*}
This enables us to identify the quantities
\begin{equation*}
    \boldsymbol{b}_k = \begin{bmatrix}\biaszero\\\biask\end{bmatrix}
        + 
        \mathbf{\Gamma} \mathbf{J} \begin{bmatrix}\pibias_{\midpoint| 0, k} \\ \pibias_{\midpoint| 0, k}\end{bmatrix},
    \quad
    \mathbf{B}_k = \mathbf{\Gamma} \mathbf{J} \mathbf{K},
    \quad
    \mathbf{\Gamma}_k = \mathbf{\Gamma}
    \eqsp.
\end{equation*}

% Therefore, we deduce the expression of  $\QMzero_k, \QNzero_k, \Qcovzero_k$, and $\Qbiaszero_k$

% \begin{align*}
%     \Qcovzero_k
%         & = \cov_{0|\tau} + (\acp{\tau}/\var_{\tau}^2) \cov_{0|\tau} \picov_{\midpoint|0,k}\cov_{0|\tau}, \\
%     \QMzero_k
%         & = (\sqrt{\acp{\tau}}/\var_{\tau}) \cov_{0|\tau} \pizero_{\midpoint| 0, k},
%     \qquad
%     \QNzero_k
%         = (\sqrt{\acp{\tau}}/\var_{\tau}) \cov_{0|\tau} \pik_{\midpoint| 0, k}, \\
%     \Qbiaszero_k
%         & = (\sqrt{\acp{\tau}}/\var_{\tau}) \cov_{0|\tau} \pibias_{\midpoint| 0, k} + \cov_{0|\tau} \cov^{-1} \mean
% \end{align*}
% and $\QMk_k, \QNk_k, \Qcovk_k$, and $\Qbiask_k$
% \begin{align*}
%     \Qcovk_k
%         & = \var_{k | \midpoint} \Id_{\dimx} + (\acp{k}/\acp{\midpoint}) \picov_{\midpoint| 0, k},\\
%     \QMk_k
%         & = \sqrt{\acp{k}/\acp{\midpoint}} \pizero_{\midpoint| 0, k},
%     \qquad
%     \QNk_k
%         = \sqrt{\acp{k}/\acp{\midpoint}} \pik_{\midpoint| 0, k},
%     \\
%     \Qbiask_k
%         & = \sqrt{\acp{k}/\acp{\midpoint}} \pibias_{\midpoint| 0, k}.
% \end{align*}

Similarly for the kernel $\lastKernel$ \eqref{eq:last-kernel-gauss}, we have
\begin{equation*}
    \begin{aligned}
        \potn{}{\bx_1} \bw{1|2}{\bx_2}{\bx_1}
            & = \normpdf(\obs; \bfA \bx_1, \stdobs^2 \Id_\dimobs) \ \fwtrans{1 | 0, 2}{\predx{2}(\bx_2), \bx_2}{\bx_1} \\
            & = \normpdf \Big(\bx_1;
                \Lcovbefore \big((1/\stdobs^2) \bfA^\top \obs + (1/\var_{1|0, 2}) (a \predx{2}(\bx_2) + b \bx_2) \big),
                \Lcovbefore
            \Big)\\
            & = \normpdf \Big(\bx_1;
                \LHbefore \bx_2 + \Lbiasbefore,
                \Lcovbefore
             \Big)
    \end{aligned}
\end{equation*}
where
\begin{align*}
    \Lcovbefore 
        & = \big[ (1/\var_{1|0, 2}) \Id_\dimx + (1/\stdobs^2) \bfA^\top\bfA \big]^{-1},
        \\
    \LHbefore
        & =  \Lcovbefore \big(
            (\sqrt{\acp{2}}/(\var_{2}\var_{1|0,2})) a \cov_{0|2} + (b/\var_{1|0,2}) \Id
            \big),
        \\
    \Lbiasbefore
        & = \Lcovbefore \big( (1/\stdobs^2) \bfA^\top \obs + (a/\var_{1|0,2}) \cov_{0|2}\cov^{-1} \mean \big)
\end{align*}

The last kernel \eqref{eq:algo-last-kernel} involves $\delta_{\predx{1}(\bx_1)}(\bx_0)$, hence, we plug the expression $\bx_1$ as a function of $\bx_0$
\begin{align*}
    \bx_0 = \predx{1}(\bx_1) \implies \bx_1 = (\var_1 / \sqrt{\acp{1}}) (\cov_{0|1}^{-1} \bx_0 - \cov^{-1} \mean)
    \eqsp,
\end{align*}
into the previous expression to obtain
\begin{align*}
    \Lcov
        & = (\acp{1}/ \var_1^2) \cov_{0|1} \ \Lcovbefore \ \cov_{0|1},
    \qquad
    \LH
        = (\sqrt{\acp{1}}/ \var_1) \cov_{0|1} \LHbefore,\\
    \Lbias
        & = (\sqrt{\acp{1}}/ \var_1) \cov_{0|1} (\Lbiasbefore + (\var_1/\sqrt{\acp{1}}) \cov^{-1}\mean).
\end{align*}

% --- redef notation to not impact the rest of the document
\renewcommand{\hpotn}[2]{\ifthenelse{\equal{#2}{}}{\hat{g}^\param _{#1}}{\hat{g}^\param _{#1}(#2)}}
% ---
