# Supplementary material for: A Mixture-Based Framework for Guiding Diffusion Models
Source: arXiv:2502.03332 source file (2025-02-05)
Supplement: Supplementary file 3 [file transition_kernels.tex]

\section{Transition kernels involved in \Cref{algo:midpoint-gibbs}}
\label{apdx:transition-kernels}
% --- local vars ---
\def\gibbsRepKernel{{Q}}
\def\initKernel{{I}}
\def\gibbsKernel{{G}}
\def\lastKernel{{L}}

% \newcommandx{\gibbsRepKernel}[1][1=\midpoint]{{Q}_{#1}}
% \newcommandx{\gibbsKernel}[1][1=\midpoint]{{G}_{#1}}
% \newcommandx{\initKernel}[1][1=k]{{I}_{#1}}
% ---

The transition kernel of one repetition of a Gibbs step reads
\begin{equation}
    \label{eq:gibbs-kernel-one-rep}
    \gibbsRepKernel(\bx_{\initpoint}, \bx_k; \rmd \bx_{\initpoint}', \rmd \bx_k')
        = \int
            \mgibbs{\midpoint |\initpoint, k}{\bx_\initpoint, \bx_k}{\rmd \bx_{\midpoint}}
            \mgibbs{\initpoint |\midpoint}{\bx_{\midpoint}}{\rmd \bx_\initpoint'}
            \mgibbs{k |\midpoint}{\bx_{\midpoint}}{\rmd \bx_k'}
    \eqsp,
\end{equation}
The initial kernel of the Gibbs steps writes
\begin{equation}
    \label{eq:gibbs-init-kernel}
    \initKernel(\bx_\initpoint; \rmd \bx_\initpoint', \rmd \bx_k')
        = \delta_{\bx_\initpoint}(\rmd \bx_\initpoint') \fwtrans{k|0}{\bx_{\initpoint}}{\rmd \bx_k'}
    \eqsp.
\end{equation}
Combining these two results, we deduce the transition kernel of one Gibbs step after applying $\gibbsReps$ repetitions
\begin{equation}
    \label{eq:gibbs-step}
    \gibbsKernel(\bx_{\initpoint}; \rmd \bx_{\initpoint}^{(R)}, \rmd \bx_k^{(R)})
        = \int
            \initKernel(\bx_\initpoint; \rmd \bx_\initpoint^{(0)}, \rmd \bx_k^{(0)})
            \prod_{r=0}^{R-1}
            \gibbsRepKernel(\bx_{\initpoint}^{(r)}, \bx_k^{(r)}; \rmd \bx_{\initpoint}^{(r+1)}, \rmd \bx_k^{(r+1)})
    \eqsp,
\end{equation}
The last two steps of the algorithm involve the following kernel, equal up to a constant that depends only on $\bx_2$
\begin{equation}
    \label{eq:algo-last-kernel}
    \lastKernel(\bx_2; \rmd \bx_0)
        \propto\int \potn{}{\bx_1} \bw{1|2}{\bx_2}{\rmd \bx_1} \delta_{\hpredx{1}{(\bx_1)}}(\rmd \bx_0)
    \eqsp.
\end{equation}
Finally, we deduce the simulated distributionx
\begin{equation*}
    \pibw{0}{}{}[\gibbsReps](\rmd \bx_0)
    % \algoKernel(\bx_n; \rmd \bx_0)
        = \int
            \fwmarg{n}{\rmd \bx _n}
            \delta_{\hpredx{n}{(\bx_n)}}(\rmd \bx_0^{n})
            \big[
                \prod_{k=2}^{n-1} \gibbsKernel(\bx_0^{k+1}; \rmd \bx_0^{k}, \rmd \bx_{k})
            \big]
            \lastKernel(\bx_2; \rmd \bx_0)
    \eqsp.
\end{equation*}
